# Supplementary material for: ADMET-EvO: a self-evolving scientific agent for sustained research across heterogeneous tasks
Source: arXiv:2609.10121 source file (2026-09-10)
Supplement: Supplementary file 1 [file supplementary.tex]

\documentclass{valhalla}
\input{styles/admet}
\begin{document}
\input{supplementary/content}
\end{document}
